# Supplementary material for: Coupled Neural Associative Memories
Source: arXiv:1301.1555 source file (2013-08-23)
Supplement: Supplementary file 1 [file appendix.tex]

\subsection{Proof of Lemma~\ref{lem:recursive}}
Let $z^{(\ell)}(t)$ denote the \emph{average} probability of error for pattern nodes across neural plane $\ell$ and in iteration $t$. Furthermore, let $\pi^{(\ell)}(t)$ be the \emph{average} probability of a \emph{custer} neuron in plane $\ell$ sending an erroneous message to its neighbors. We will derive recursive expressions for $z^{(\ell)}(t)$ and $\pi^{(\ell)}(t)$. 

A cluster node in plane $\ell$ receives noisy messages from its neighbors with an average probability of $\bar{z}^{(\ell)}$, where 
$$\bar{z}^{(\ell)} = \frac{1}{2\Omega+1}\sum_{j=-\Omega}^{\Omega} z^{(\ell-j)}$$
with $z^{(i)} = 0$ for $i \leq 0$ and $i > L$. 

Let $\pi_i^{(\ell)}$ denote the the probability that a cluster node with degree $i$ in plane $\ell$ sends an erroneous message to its neighboring pattern nodes. Then, knowing that each cluster is capable of correcting at least one error, $\pi_i^{(\ell)}$ is equal to the probability of receiving two or more noisy messages from pattern neurons,
$$\pi_i^{(\ell)} = 1-\left(1-\bar{z}^{(\ell)}\right)^{i}-i \bar{z}^{(\ell)} \left(1-\bar{z}^{(\ell)}\right)^{i-1}.$$
Now, letting $\pi^{(\ell)}(t)$ denote the average probability of sending erroneous nodes by cluster nodes in plane $\ell$ and in iteration $t$, we will have
\begin{eqnarray*}
\pi^{(\ell)}(t) &=& \mb{E} \{\pi_i^{(\ell)}\}\\ &=& \sum_{i} \rho_{i} \pi_i^{(\ell)} \\
&=& 1-\rho(1-\bar{z}^{(\ell)}(t))+\bar{z}^{(\ell)}(t)\rho'(1-\bar{z}^{(\ell)}(t)),
\end{eqnarray*}
where $\rho(z) = \sum_i \rho_i z^i$ is the cluster node degree distribution polynomial and $\rho'(z) = d\rho(z)/dz$. %Note that the above equation is very similar to the peeling decoder recursion in correcting erasures \cite{erasure}, except for the additional $\bar{z}^{(\ell)}(t)\rho'(1-\bar{z}^{(\ell)}(t))$ term which comes from the capability of each cluster to correct one error. 

To simplify notations, let us define the function $g(z)=1-\rho(1-z)+z\rho'(1-z)$ such that
$$\pi^{(\ell)}(t) = g(\bar{z}^{(\ell)}(t)).$$
Now consider a given pattern neuron with degree $j$ in plane $\ell$. In iteration $t+1$, Let $z_j^{(\ell)}(t)$ denote the probability of sending an erroneous message by this node. Then, $z_j^{(\ell)}(t)$ is equal to the probability of this node being noisy in the first place ($p_e$) and having all its cluster nodes sending erroneous messages in iteration $t$, the average probability of which is $$\bar{\pi}^{(\ell)}(t)=\frac{1}{2\Omega + 1}\sum_{i=-\Omega}^{\Omega}\pi^{(\ell-i)}(t).$$ Now, since $z^{(\ell)}(t+1) = \mb{E} \{z_j^{(\ell)}(t+1)\}$, we get
\beqa
z^{(\ell)}(t+1) &=& p_e \sum_j \lambda_j \left( \bar{\pi}^{(\ell)} \right)^{j} \nonumber \\
%&=& \lambda\left( \bar{\pi}^{(\ell)} \right) \nonumber \\
&=&p_e \lambda(\bar{\pi}^{(\ell)}) \nonumber \\
&=& p_e \lambda(\frac{1}{2\Omega + 1}\sum_{i=-\Omega}^{\Omega}g(\bar{z}^{(\ell-i)}(t))\nonumber
\eeqa

Again to simplify the notation, let us define the function $f(z;p_e) = p_e \lambda(z)$. This way, we will have the recursion as:
$$z^{(\ell)}(t+1) = f(\frac{1}{2\Omega + 1}\sum_{i=-\Omega}^{\Omega}g(\bar{z}^{(\ell-i)}(t);p_e).$$

\subsection{Proof of Theorem~\ref{lemma:unconstrained_coupled}}
The proof is straightforward and results from the definition of the potential. Because of the definition of $p_e^\dagger$, we know that for $p_e \leq p_e^\dagger$ we have $$U'(\textbf{z};p_e) > 0.$$ From equation (\ref{eq:potential}), we have $$U'(\textbf{z};p_e) = \textbf{g}'(\textbf{z})(\textbf{z}-A^\top \textbf{f}(A\textbf{g}(\textbf{z})).$$ Given that $\textbf{g}'(\textbf{z}) >0$, from $U'(\textbf{z};p_e) > 0$ we conclude that $$\textbf{z}-A^\top \textbf{f}(A\textbf{g}(\textbf{z}))>0.$$ This is equivalent to saying that 
\bed
z^{(\ell)}(t+1) = A^\top \textbf{f}(A\textbf{g}(\textbf{z}^{(\ell)}(t)))< z^{(\ell)}(t).
\eed
Therefore,$$z^{(\ell)}(t)\rightarrow 0,\forall \ell.$$ 

\subsection{Proof of Theorem~\ref{theorem:constrained_coupled}}
The proof of the theorem relies on results from \cite{kudekar} to show that the entries in the vector $\textbf{z}(t) = [z^{(1)}(t),\dots,z^{(L)}(t)]$ are non-decreasing, i.e.,  $$z^{(1)}(t)\leq z^{(2)}(t)\leq \dots \leq z^{(L)}(t).$$ This can be shown using induction and the the functions $\textbf{f}(\cdot,p_e)$ and $\textbf{g}(\cdot)$ are non-decreasing (see the proof of Lemma 22 in \cite{kudekar} for more details).

Then, one can apply the result of Lemma 3 in \cite{pfister_istc} to show that the potential function of the constrained coupled system decreases in each iteration. Finally, when $$L > \Vert U''(\textbf{z};p_e)\Vert_{\infty} / \Delta E(p_e)$$ one could apply Theorem 1 of \cite{pfister_istc} to show the convergence of the probability of errors to zero.

\subsection{Proof of Theorem~\ref{theorem_exponential_solution}}
The proof is based on construction: we construct a data set $\mc{X}$ with the required properties such that it can be memorized by the proposed neural network. To simplify the notations, we assume all the clusters have the same number of pattern and constraint neurons, denote by $\tilde{n}_c$ and $\tilde{m}_c$. In other words, $n_{\ell,d} = \tilde{n}_c$ and $m_{\ell,d} = \tilde{m}_c $ for all $\ell=\{1,\dots,L\}$and $d=\{1,\dots,D\}$.

We start by considering a matrix $G \in \mb{R}^{k \times n}$, with non-negtaive integer-valued entries between $0$ and $\gamma-1$ for some $\gamma \geq 2$. We also assume $k = rn$, with $0 < r < 1$.

To construct the database, we first divide the columns of $G$ into $L$ sets, each corresponding to the neurons in one plain. Furthermore, in order to ensure that all the sub-patterns within each cluster for a supspace with dimension less than $\tilde{n}_c$, we propose the following structure for the generator matrix $G$. This strucutre ensures that the rank of any sub-matrix of $G$ composed of $\tilde{n}_c$ columns is less than $\tilde{n}_c$. In the matrices below, the hatched blocks represent parts of the matrix with \emph{some} non-zero entries. To simplfiy visualization, let us first define the sub-matrix $\hat{G}$ as the building blocks of $G$:
\vspace{-1.3cm}
\begin{center}
\begin{tikzpicture}[scale=1]
%\tikzstyle{every node}=[draw]
%\matrix [draw = white,left delimiter=(,right delimiter=)]
%{
\node at (0,0)[yshift=-2.1cm,xshift=0] (v0) {$\hat{G}=$};
\node at (0,0)[yshift=-2.1cm,xshift=3.1cm,rectangle,minimum size=42mm,left delimiter={[}] (v1) {};
\node at (0,0)[yshift=-2.1cm,xshift=2.7cm,rectangle,minimum size=42mm,right delimiter={]}] (v2) {};
\draw[pattern=north west lines][xshift=1cm] (0,0)--(1.5,0)--(1.5,-0.75)--(2.25,-0.75)--(2.25,-1.5)--(3,-1.5)--(3,-2.25)--(3.75,-2.25)--(3.75,-3.75)--(2.25,-3.75)--(2.25,-3)--(1.5,-3)--(1.5,-2.25)--(0.75,-2.25)--(0.75,-1.5)--(0,-1.5)--cycle;
\node at (1.5,1.3)[yshift=-.15cm,xshift=0.25cm,rectangle,minimum size=15mm,below delimiter=\{] (v3) {};
\node at (1.5,1.3)[yshift=-.6cm,xshift=0.25cm] (v8) {$n/(D\cdot L)$};
\node at (-1.8,-.65)[yshift=-3.5,xshift=1.5cm,rectangle,minimum size=15mm,right delimiter=\{] (v4) {$k/(D\cdot L)$};
%\node at (1.2,0)[yshift=-3,xshift=1.75cm,rectangle,minimum size=4.6mm,below delimiter=\{] (v0) {$\Delta n$};
\end{tikzpicture}
\end{center}

Then, $G$ is structured as
\begin{center}
\begin{tikzpicture}[scale=0.25]
%\tikzstyle{every node}=[draw]
%\matrix [draw = white,left delimiter=(,right delimiter=)]
%{
%\draw[help lines] (-9,-9) grid (9,9); 
\node at (-11,2)(v0) {$G$=};
\node at (-2,1.8)[rectangle,minimum size=34mm,left delimiter={[}] (v1) {};
\node at (2,1.8)[rectangle,minimum size=34mm,right delimiter={]}] (v2) {};
\node at (-6.8,6.3)[rectangle,minimum size=10mm,pattern=north west lines] (v2) {};
\draw[-,dashed](-4.6,8.7)--(-4.6,-5);
\node at (-2.3,6.3)[rectangle,minimum size=10mm,pattern=north west lines] (v2) {};
\draw[-,dashed](0.1,8.7)--(-.1,-5);
\node at (-2.3,1.8)[rectangle,minimum size=10mm,pattern=north west lines] (v2) {};
\draw[-,dashed](4.4,8.7)--(4.4,-5);
\node at (2.2,1.8)[rectangle,minimum size=10mm,pattern=north west lines] (v2) {};
\node at (2.2,-2.7)[rectangle,minimum size=10mm,pattern=north west lines] (v2) {};
\node at (6.7,-2.7)[rectangle,minimum size=10mm,pattern=north west lines] (v2) {};
\draw[-,dashed](-8.9,4.1)--(8.9,4.1);
\draw[-,dashed](-8.9,-.4)--(8.9,-.4);
\end{tikzpicture}
\end{center}
where each hatched block represents a random realization of $\hat{G}$.

Now consider a random vector $u \in \mb{R}^k$ with integer-valued-entries between $0$ and $\upsilon-1$, where $\upsilon \geq 2$. We construct the dataset by assigning the pattern $\textbf{x} \in \mc{X}$ to be $\textbf{x} = \textbf{u} \cdot G$, \emph{if} all the entries of $\textbf{x}$ are between $0$ and $S-1$. Obviously, since both $\textbf{u}$ and $G$ have only non-negative entries, all entries in $\textbf{x}$ are non-negative. Therefore, it is the $S-1$ upper bound that we have to worry about. 

Let $\varrho_j$ denote the $j^{th}$ column of $G$. Then the $j^{th}$ entry in $\textbf{x}$ is equal to $x_j = \textbf{u} \cdot \varrho_j$. Suppose $\varrho_j$ has $d_j$ non-zero elements. Then, we have: 
\bed
x_j = u \cdot \varrho_j \leq d_j (\gamma-1) (\upsilon-1)
\eed

Therefore, letting $d^* = \max_{j} d_j$, we could choose $\gamma$, $\upsilon$ and $d^*$ such that
\beq\label{capaci_inequal}
S-1 \geq d^* (\gamma-1) (\upsilon-1)
\eeq
to ensure all entries of $x$ are less than $S$. 

As a result, since there are $\upsilon^k$ vectors $u$ with integer entries between $0$ and $\upsilon -1$, we will have $\upsilon^k = \upsilon^{rn}$ patterns forming $\mc{X}$. Which means $\mc{C} = \upsilon^{rn}$, which would be an exponential number in $n$ if $\upsilon \geq 2$.
